# Supplementary material for: Stock Price Responses to Firm-Level News in Supply Chain Networks
Source: arXiv:2409.06255 source file (2026-01-14)
Supplement: Supplementary file 1 [file SI.pdf]

# Market Reaction to News Flows in Supply Chain Networks

## Supplementary Information

Hiroyasu Inoue and Yasuyuki Todo

### 1 Supplementary tables

The following is the list of tables referred to in the main text.

SI Table 1: Difference between the post- and pre-news effect of the disclosure of negative news articles about firms across the world on their suppliers' stock prices.

SI Table 2: Difference between the post- and pre-news effect of the disclosure of negative news articles about firms across the world on their client' stock prices.

SI Table 1: Difference between the post- and pre-news effect of the disclosure of negative news articles about firms across the world on their suppliers' stock prices.  $P$  values are those from  $t$  tests for the null hypothesis that the difference is 0. \*\*\*, \*\*, and \* indicate statistical significance at the 1, 5, and 10% level, respectively.

| Time window (days)               | 1         | 2         | 3         | 4         | 5        | 30       | 180      | 365      |
|----------------------------------|-----------|-----------|-----------|-----------|----------|----------|----------|----------|
| $\beta_w^{post} - \beta_w^{pre}$ | -0.017*** | -0.014*** | -0.010*** | -0.005*** | -0.001** | 0.001*** | 0.002*** | 0.001*** |
| $p$ value                        | 0.00      | 0.00      | 0.00      | 0.00      | 0.02     | 0.00     | 0.00     | 0.00     |

SI Table 2: Difference between the post- and pre-news effect of the disclosure of negative news articles about firms across the world on their client' stock prices.  $P$  values are those from  $t$  tests for the null hypothesis that the difference is 0. \*\*\*, \*\*, and \* indicate statistical significance at the 1, 5, and 10% level, respectively.

| Time window (days)               | 1         | 2         | 3         | 4         | 5         | 30       | 180       | 365       |
|----------------------------------|-----------|-----------|-----------|-----------|-----------|----------|-----------|-----------|
| $\beta_w^{post} - \beta_w^{pre}$ | -0.014*** | -0.016*** | -0.013*** | -0.008*** | -0.005*** | 0.001*** | -0.003*** | -0.001*** |
| $p$ value                        | 0.00      | 0.00      | 0.00      | 0.00      | 0.00      | 0.00     | 0.00      | 0.00      |
